# Supplementary material for: RISE-iEEG: Robust to Inter-Subject Electrodes Implantation Variability iEEG Classifier
Source: arXiv:2408.14477 source file (2025-04-15)
Supplement: Supplementary file 1 [file Appendix.tex]

% Prefix table numbers with "A" in the appendix
\setcounter{table}{0} % Reset the table counter for the appendix
 % Prefix figure numbers with "A" in the appendix
\setcounter{figure}{0} % Reset the figure counter for the appendix
\section{}

\subsection{Finding the Significant Lobe}
\label{significant lobe}
First, we calculate the Integrated Gradients (IG) for the data of each trial \(i\) from each participant \(p\), represented as \( \text{IG}_i^p \). This is a 2D matrix in which each row corresponds to the IG values of a specific electrode over time. As explained in section \ref{IG method}, the IG values indicate the contribution (or importance) of the data in predicting the label. Subsequently, we apply Algorithm \ref{alg:important_lobe} to identify the significant lobe (\( \text{SL}_p^i \)) for each participant.

\begin{algorithm}[h]
\caption{Finding the Significant Lobe Based on IG}
\label{alg:important_lobe}
\begin{algorithmic}[1]
\REQUIRE 
   Integrated Gradients $\text{IG}_i^p \in \mathbb{R}^{\text{Ch} \times T}$ for each trial $i$ of each participant $p$, where $\text{Ch}$ is the number of electrodes and $T$ is the number of time samples.
\ENSURE
    Significant lobe for each participant ($\text{SL}^p$).

\FOR{each participant $p$}
    \FOR{each trial $i$}
        \FOR{each electrode $j$}
            \STATE Sum IG along the time axis: $\text{IG}_{i,j}^p = \sum_{t=1}^{T} \text{IG}_{i,j,t}^p$
        \ENDFOR
        \STATE Identify the electrode $j^*$ with the highest $\text{IG}_{i,j}^p$.
        \STATE Assign the brain region of electrode $j^*$ as the significant lobe ($\text{SL}_{i}^p$).
    \ENDFOR
\ENDFOR

\FOR{each participant $p$}
    \STATE Apply majority voting across $\text{SL}_{i}^p$ to find the significant lobe ($\text{SL}^p$).
\ENDFOR

\STATE \textbf{Return} Significant lobe for each participant ($\text{SL}^p$).
\end{algorithmic}
\end{algorithm}

%%%%%%%%%%%%%%%%%%%%%%%%%%%%%%%%%%%%%%%%%%%%%%%%%%%%%%%%%%%%
\subsection{Significant Lobe Analysis via Integrated Gradients}
\label{select_three_lobes}
In this analysis, we rank brain regions based on their IG (Integrated Gradients) values, which indicate the importance of each region in predicting the label. We present the variation in IG across these ranked brain regions in Figs. \ref{curve_lobe_sm} and \ref{curve_lobe_mr} for the 'Singing vs. Music' and 'Move vs. Rest' tasks, respectively. As shown in these figures, for most participants, around 80\% of the IG information is, on average, contained within the first three lobes.
\begin{figure*}[t]
	\centering
	\includesvg[width =\textwidth]{figs/Curves_best_lobes_subplot_Singing_music.svg}
	\caption{Distribution of IG information across brain lobes for participants in the 'Singing vs. Music' task. Each subplot represents the percentage of IG information associated with brain lobes ranked by their contribution to model predictions. The red stars indicate the 'knee points,' which signify the optimal cutoff where adding more lobes provides minimal additional predictive value. This threshold highlights the most critical lobes for distinguishing between singing and music tasks for each participant.}
	\centering
	\label{curve_lobe_sm}
\end{figure*}

\begin{figure*}[t]
	\centering
	\includesvg[width =\textwidth]{figs/Curves_best_lobes_subplot_move_rest.svg}
	\caption{Distribution of IG information across brain lobes for participants in the Move vs. Rest task. Each subplot represents the percentage of IG information associated with brain lobes ranked by their contribution to model predictions. The red stars indicate the 'knee points,' which signify the optimal cutoff where adding more lobes provides minimal additional predictive value. This threshold highlights the most critical lobes for distinguishing between singing and music tasks for each participant.}
	\centering
	\label{curve_lobe_mr}
\end{figure*}

%%%%%%%%%%%%%%%%%%%%%%%%%%%%%%%%%%%%%%%%%%%%%%%%%%%%%%%%%%%
\subsection{Analyze the weights of projection network}

\begin{table}[ht]
\centering
\caption{The lobe brain with the highest weight in participant-specific projection layer for each participant in the 'Move vs. Rest' task.}
 % Adjust row spacing for compactness
\begin{tabular}{c c c c}
\hline
\textbf{Participant} & \textbf{Lobe} & \textbf{Participant} & \textbf{Lobe} \\ \hline

\textbf{1} & Inferior Temporal & \textbf{7} & \textcolor[HTML]{CB0000}{Postcentral} \\

\textbf{2} & \textcolor[HTML]{CB0000}{Precentral} & \textbf{8} & Supramarginal \\

\textbf{3} & \textcolor[HTML]{CB0000}{Postcentral} & \textbf{9} & Temporal Pole \\

\textbf{4} & \textcolor[HTML]{CB0000}{Postcentral} & \textbf{10} & Superior Temporal \\

\textbf{5} & Temporal Pole & \textbf{11} & \textcolor[HTML]{CB0000}{Postcentral} \\

\textbf{6} & Superior Parietal & \textbf{12} & \textcolor[HTML]{CB0000}{Precentral} \\
\hline
\end{tabular}
\label{tab:weight2}
\end{table}

\begin{table}[ht]
\centering
\caption{The lobe brain with the highest weight in participant-specific projection layer for each participant in the 'Singing vs. Music' task.}
 % Adjust row spacing for compactness
\begin{tabular}{c c c c}
\hline
\textbf{Participant} & \textbf{Lobe} & \textbf{Participant} & \textbf{Lobe} \\ \hline

\textbf{1} & \textcolor[HTML]{CB0000}{Superior temporal} & \textbf{15} & \textcolor[HTML]{CB0000}{Superior temporal} \\

\textbf{2} & \textcolor[HTML]{CB0000}{Superior temporal} & \textbf{16} & Precentral \\

\textbf{3} & \textcolor[HTML]{CB0000}{Superior temporal} & \textbf{17} & \textcolor[HTML]{CB0000}{Superior temporal} \\

\textbf{4} & \textcolor[HTML]{CB0000}{Superior temporal} & \textbf{18} & \textcolor[HTML]{CB0000}{Superior temporal} \\

\textbf{5} & \textcolor[HTML]{CB0000}{Superior temporal} & \textbf{19} & \textcolor[HTML]{CB0000}{Superior temporal} \\

\textbf{6} & \textcolor[HTML]{CB0000}{Superior temporal} & \textbf{20} & \textcolor[HTML]{CB0000}{Superior temporal} \\

\textbf{7} & \textcolor[HTML]{CB0000}{Superior temporal} & \textbf{21} & Rostral middle frontal \\

\textbf{8} & \textcolor[HTML]{CB0000}{Superior temporal} & \textbf{22} & \textcolor[HTML]{CB0000}{Superior temporal} \\

\textbf{9} & Precentral & \textbf{23} & Inferior temporal \\

\textbf{10} & \textcolor[HTML]{CB0000}{Superior temporal} & \textbf{24} & \textcolor[HTML]{CB0000}{Superior temporal} \\

\textbf{11} & Superior frontal & \textbf{25} & \textcolor[HTML]{CB0000}{Superior temporal} \\

\textbf{12} & Precentral & \textbf{26} & \textcolor[HTML]{CB0000}{Superior temporal} \\

\textbf{13} & Pars orbitalis & \textbf{27} & \textcolor[HTML]{CB0000}{Superior temporal} \\

\textbf{14} & \textcolor[HTML]{CB0000}{Superior temporal} & \textbf{28} & Supramarginal \\

    &                          & \textbf{29} & \textcolor[HTML]{CB0000}{Superior temporal} \\
\hline
\end{tabular}
\label{tab:weight}
\end{table}

\subsection{ROC curves}
Fig.\ref{roc} presents the ROC curve for each task, illustrating the model's classification performance and highlighting the trade-off between true positive and false positive rates across different decision thresholds.

\begin{figure*}[t]
	\centering
	\includesvg[width = \textwidth]{figs/ROC.svg}
	\caption{ROC curves for (A) 'Move vs. Rest' task and (B) 'Singing vs. Music' task.}
	\centering
	\label{roc}
\end{figure*}
